# Supplementary material for: RanDeS: Randomized Delta Superposition for Multi-Model Compression
Source: arXiv:2505.11204 source file (2025-05-16)
Supplement: Supplementary file 2 [file 7_appendix_deprecated.tex]

 % \newpage
% \appendix
% \input{s1_overview}
% \input{s2_datasheet}
% \input{s3_dataset}
% \input{s4_experiments}

% TODO: outline paper finish by EOD Thursday.

% TODO thread 2: finish content bottom up.
% experiment with empty tables.

% abstract

% ablation: superposed model soup, two aspects. all the things I tried.

% story

% method

% discussion

% intro

% \begin{figure}[h]
%     \centering
%     \includegraphics[width=1.0\textwidth]{images/four_similarity_matrices_gpt2.pdf}
%     \vspace{-4mm}
%     \caption{Pairwise cosine similarity comparison of target layers on GPT-2 models between superposed and original task vectors, with and without layer shifting. (TODO: make the font size larger)}
%     \label{fig:pairwise_consine_similarity_sta}
%     \vspace{-1mm}
% \end{figure}

% \section{Superposition Leads to Zero Pairwise Cosine Similarity in Expectation}


% % All artwork must be neat, clean, and legible. Lines should be dark
% % enough for purposes of reproduction; art work should not be
% % hand-drawn. The figure number and caption always appear after the
% % figure. Place one line space before the figure caption, and one line
% % space after the figure. The figure caption is lower case (except for
% % first word and proper nouns); figures are numbered consecutively.

% % Make sure the figure caption does not get separated from the figure.
% % Leave sufficient space to avoid splitting the figure and figure caption.

% % You may use color figures.
% % However, it is best for the
% % figure captions and the paper body to make sense if the paper is printed
% % either in black/white or in color.
% % \begin{figure}[h]
% % \begin{center}
% % %\framebox[4.0in]{$\;$}
% % \end{center}
% % \caption{Sample figure caption.}
% % \end{figure}


% \begin{definition}[Matrix Cosine Similarity]
%     The cosine similarity between two matrices $\bm{A}$ and $\bm{B}$ is defined as $\cos(\bm{A},\bm{B})=\frac{\langle \bm{A},\bm{B}\rangle_F}{\|\bm{A}\|_F\|\bm{B}\|_F}$, where $\langle\cdot,\cdot\rangle_F$ and $\|\cdot\|_F$ are the Frobenius inner product and Frobenius norm respectively. It's equivalent to the cosine similarity of two matrices after vectorization.
% \end{definition}



% \begin{theorem}
%     Let $\bm{A}, \bm{B} \in \mathbb{R}^{m \times n}$ be two arbitrary matrices. Let $\bm{D}_1$ and $\bm{D}_2$ be independent random diagonal matrices whose diagonal entries are independent Rademacher random variables (i.e., each diagonal entry is independently $\pm 1$ with equal probability). Then:

%     The expected cosine similarity between $\bm{A} \bm{D}_1$ and $\bm{B} \bm{D}_2$ is zero:
%     \[
%     \mathbb{E}[\cos(\bm{A} \bm{D}_1, \bm{B} \bm{D}_2)] = 0.
%     \]
%     The variance of the cosine similarity is given by:
%     \[
%     \mathrm{Var}(\cos(\bm{A} \bm{D}_1, \bm{B} \bm{D}_2)) = \frac{\sum_{i,j} (A_{i,j} B_{i,j})^2}{\|\bm{A}\|_F^2 \|\bm{B}\|_F^2}.
%     \]
% \end{theorem}


% \begin{proof}
    
% \textbf{1. Expected Cosine Similarity is Zero}

% The cosine similarity between $\bm{A} \bm{D}_1$ and $\bm{B} \bm{D}_2$ is defined as:
% \[
% \cos(\bm{A} \bm{D}_1, \bm{B} \bm{D}_2) = \frac{\langle \bm{A} \bm{D}_1, \bm{B} \bm{D}_2 \rangle_F}{\|\bm{A} \bm{D}_1\|_F \|\bm{B} \bm{D}_2\|_F}.
% \]
% Since $\bm{D}_1$ and $\bm{D}_2$ are orthogonal matrices (diagonal with $\pm 1$ entries), they preserve the Frobenius norm:
% \[
% \|\bm{A} \bm{D}_1\|_F = \|\bm{A}\|_F, \quad \|\bm{B} \bm{D}_2\|_F = \|\bm{B}\|_F.
% \]
% Thus,
% \[
% \cos(\bm{A} \bm{D}_1, \bm{B} \bm{D}_2) = \frac{\langle \bm{A} \bm{D}_1, \bm{B} \bm{D}_2 \rangle_F}{\|\bm{A}\|_F \|\bm{B}\|_F}.
% \]
% Compute the expected inner product in the numerator:
% \[
% \mathbb{E}[\langle \bm{A} \bm{D}_1, \bm{B} \bm{D}_2 \rangle_F] = \sum_{i,j} A_{i,j} B_{i,j} \mathbb{E}[(D_1)_{j,j} (D_2)_{j,j}].
% \]
% Since $(D_1)_{j,j}$ and $(D_2)_{j,j}$ are independent Rademacher variables with zero mean:
% \[
% \mathbb{E}[(D_1)_{j,j} (D_2)_{j,j}] = \mathbb{E}[(D_1)_{j,j}] \mathbb{E}[(D_2)_{j,j}] = 0.
% \]
% Therefore,
% \[
% \mathbb{E}[\langle \bm{A} \bm{D}_1, \bm{B} \bm{D}_2 \rangle_F] = 0,
% \]
% and thus,
% \[
% \mathbb{E}[\cos(\bm{A} \bm{D}_1, \bm{B} \bm{D}_2)] = 0.
% \]

% \textbf{2. Variance of the Cosine Similarity}

% Since the denominator \( \|\bm{A}\|_F \|\bm{B}\|_F \) is constant, the variance of the cosine similarity is:
% \[
% \mathrm{Var}(\cos(\bm{A} \bm{D}_1, \bm{B} \bm{D}_2)) = \frac{\mathrm{Var}(\langle \bm{A} \bm{D}_1, \bm{B} \bm{D}_2 \rangle_F)}{\|\bm{A}\|_F^2 \|\bm{B}\|_F^2} = \frac{\mathrm{Var}(X)}{\|\bm{A}\|_F^2 \|\bm{B}\|_F^2}.
% \]
% To compute \( \mathrm{Var}(X) \), since \( \mathbb{E}[X] = 0 \), we have:
% \begin{align*}
%     \mathrm{Var}(X) &= \mathbb{E}[X^2] - (\mathbb{E}[X])^2, \\
%     &= \mathbb{E}[X^2], \\
%     &=\mathbb{E}\left[\left( \sum_{i,j} A_{i,j} B_{i,j} (D_1)_{j,j} (D_2)_{j,j} \right)^2\right], \\
%     &=\sum_{i,j} \sum_{k,l} A_{i,j} B_{i,j} A_{k,l} B_{k,l} \mathbb{E}[(D_1)_{j,j} (D_2)_{j,j} (D_1)_{l,l} (D_2)_{l,l}].
% \end{align*}

% Since \( (D_1)_{j,j} \) and \( (D_2)_{j,j} \) are independent across different \( j \), and independent of each other, we consider two cases:

% - For \( j = l \), we have \( \mathbb{E}[(D_1)_{j,j}^2] = 1 \) and \( \mathbb{E}[(D_2)_{j,j}^2] = 1 \). Therefore,
% \[
% \mathbb{E}[(D_1)_{j,j}^2 (D_2)_{j,j}^2] = 1.
% \]
% - For \( j \neq l \), we have:
% \[
% \mathbb{E}[(D_1)_{j,j} (D_2)_{j,j} (D_1)_{l,l} (D_2)_{l,l}] = \mathbb{E}[(D_1)_{j,j} (D_1)_{l,l}] \mathbb{E}[(D_2)_{j,j} (D_2)_{l,l}] = 0.
% \]

% Thus, the only non-zero terms occur when \( j = l \), so:
% \[
% \mathbb{E}[X^2] = \sum_{i,j} (A_{i,j} B_{i,j})^2.
% \]
% Therefore, the variance of \( X \) is:
% \[
% \mathrm{Var}(X) = \sum_{i,j} (A_{i,j} B_{i,j})^2.
% \]
% Finally, the variance of the cosine similarity is:
% \[
% \mathrm{Var}(\cos(\bm{A} \bm{D}_1, \bm{B} \bm{D}_2)) = \frac{\mathrm{Var}(X)}{\|\bm{A}\|_F^2 \|\bm{B}\|_F^2} = \frac{\sum_{i,j} (A_{i,j} B_{i,j})^2}{\|\bm{A}\|_F^2 \|\bm{B}\|_F^2}.
% \]
% \end{proof}

% \begin{lemma}
% As $\bm{A}$ and $\bm{B}$ become more orthogonal (i.e., their entries align less), the variance of the cosine similarity decreases.
% \end{lemma}

% \begin{proof}
% The variance of the matrix cosine similarity is given by:
% \[
% \mathrm{Var}(\cos(\bm{A} \bm{D}_1, \bm{B} \bm{D}_2)) = \frac{\sum_{i,j} (A_{i,j} B_{i,j})^2}{\|\bm{A}\|_F^2 \|\bm{B}\|_F^2}.
% \]
% If $\bm{A}$ and $\bm{B}$ are more orthogonal, this implies that the entries $A_{i,j}$ and $B_{i,j}$ align less. As a result, the values of $A_{i,j} B_{i,j}$ will tend to decrease, leading to a smaller numerator in the expression for the variance. Therefore, the variance decreases as the matrices become more orthogonal.
% \end{proof}












% \begin{theorem}
%     Applying independent random binary diagonal matrices, with diagonal entries drawn from the Rademacher distribution, to a pair of arbitrary matrices reduces their expected matrix cosine similarity to zero.
% \end{theorem}
% \begin{proof}
%     Let $\bm{A}$ and $\bm{B}$ be arbitrary matrices of the same dimensions. Let $\bm{D_1}$ and $\bm{D_2}$ be independent random diagonal matrices whose diagonal entries $\varepsilon_i$ and $\delta_j$ are independent Rademacher random variables, meaning $\varepsilon_i, \delta_j$ with equal probability $\frac{1}{2}$. Note that $\bm{D_1}$ and $\bm{D_2}$ are orthogonal matrices since $\bm{D_1}^\top\bm{D_1}=\bm{I}$ and $\bm{D_2}^\top\bm{D_2}=\bm{I}$. We will show that the expected matrix cosine similarity between $\bm{AD_1}$ and $\bm{BD_2}$ is zero:
%     $$\mathbb{E}[\cos(\bm{AD_1},\bm{BD_2})]=0$$
%     By definition, the matrix cosine similarity between $\bm{AD_1}$ and $\bm{BD_2}$ is
%     $$\cos(\bm{AD_1},\bm{BD_2})=\frac{\langle \bm{AD_1},\bm{BD_2}\rangle_F}{\|\bm{AD_1}\|_F\|\bm{BD_2}\|_F}$$
%     Expand the numerator, we have:
%     $$\langle \bm{AD_1},\bm{BD_2}\rangle_F=\sum_{i,j}(D_1)_{i,i}A_{i,j}(D_2)_{j,j}B_{i,j}=\sum_{i,j}(\bm{AD_1})_{i,j}(\bm{BD_2})_{i,j}=\sum_{i,j}A_{i,j}\varepsilon_iB_{i,j}\delta_j$$
%     Since $\varepsilon_i$ and $\delta_j$ are independent with zero mean: $\mathbb{E}[\varepsilon_i]=\mathbb{E}[\delta_j]=0$. Thus,
%     $$\mathbb{E}[\langle \bm{AD_1},\bm{BD_2}\rangle_F]=\sum_{i,j}A_{i,j}\mathbb{E}[\varepsilon_i]B_{i,j}\mathbb{E}[\delta_j]=0$$
%     For the denominator, since $\bm{D_1}$ and $\bm{D_2}$ are orthogonal:
%     $$\|\bm{AD_1}\|_F=\|\bm{A}\|_F,~~~\|\bm{BD_2}\|_F=\|\bm{B}\|_F$$
%     Therefore,
%     $$\mathbb{E}[\cos(\bm{AD_1},\bm{BD_2})]=\frac{\mathbb{E}[\langle \bm{AD_1},\bm{BD_2}\rangle_F]}{\|\bm{A}\|_F\|\bm{B}\|_F}=\frac{0}{\|\bm{A}\|_F\|\bm{B}\|_F}=0$$

%     This shows that applying independent random binary diagonal matrices drawn from the Rademacher distribution to $\bm{A}$ and $\bm{B}$ reduces their expected matrix cosine similarity to zero.
    
% \end{proof}
















% \begin{theorem}
% Increasing the mutual orthogonality among a set of matrices via orthogonal transformations reduces the Frobenius norm of their sum.
% \end{theorem}

% \begin{proof}
% Let $\{A_i\}_{i=1}^n$ be non-zero matrices in $\mathbb{R}^{h \times w}$, and let $\{B_i\}_{i=1}^n$ be their orthogonally transformed counterparts: $B_i = A_i Q_i$, where each $Q_i$ is an orthogonal matrix ($Q_i^\top Q_i = I$).

% The Frobenius norm is preserved under orthogonal transformations: $\|B_i\|_F = \|A_i\|_F$. The inner product between transformed matrices satisfies $\langle B_i, B_j \rangle_F = \langle A_i Q_i, A_j Q_j \rangle_F$.

% The squared Frobenius norm of the sum is:
% \[
% \left\| \sum_{i=1}^n B_i \right\|_F^2 = \sum_{i=1}^n \|A_i\|_F^2 + 2 \sum_{i<j} \langle B_i, B_j \rangle_F.
% \]
% If the transformations increase orthogonality, then $\langle B_i, B_j \rangle_F \leq \langle A_i, A_j \rangle_F$. Therefore,
% \[
% \left\| \sum_{i=1}^n B_i \right\|_F^2 \leq \sum_{i=1}^n \|A_i\|_F^2 + 2 \sum_{i<j} \langle A_i, A_j \rangle_F = \left\| \sum_{i=1}^n A_i \right\|_F^2.
% \]
% Thus, increasing mutual orthogonality reduces the Frobenius norm of the sum.
% \end{proof}

\section{Derivation of \hyperref[interference_frob_norm_equation]{Equation~\ref*{interference_frob_norm_equation}}} \label{interference_frob_norm_derivation}
Here we derive the squared Frobenius norm of the interference $\lambda\sum_{i\neq k}\bm{T}_i^k$ in more details:
\begin{align}
    \left\|\lambda\sum_{i\neq k}\bm{T}_i^k\right\|_F^2 &= \left\langle\lambda\sum_{i\neq k}\bm{T}_i^k,\lambda\sum_{i\neq k}\bm{T}_i^k\right\rangle_F, \\
    &=\lambda^2\left(\sum_{i\neq k}\sum_{j\neq k}\langle\bm{T}_i^k, \bm{T}_j^k\rangle_F\right), \\
    &= \lambda^2\left(\sum_{i\neq k}\langle\bm{T}_i^k,\bm{T}_i^k\rangle_F + \sum_{i,j\neq k}\langle\bm{T}_i,\bm{T}_j^k\rangle_F\right),\\
    &= \lambda^2\left(\sum_{i\neq k}\|\bm{T}_i^k\|_F^2+2\sum_{\substack{1 \leq i < j \leq n \\ i, j \neq k}}\langle\bm{T}_i^k,\bm{T}_j^k\rangle_F \right),\\
    &= \lambda^2\left(\sum_{i\neq k}\|\bm{T}_i^k\|_F^2+2\sum_{\substack{1 \leq i < j \leq n \\ i, j \neq k}}\|\bm{T}_i^k\|_F\|\bm{T}_j^k\|_F\cos(\bm{T}_i^k,\bm{T}_j^k)\right).
\end{align}

% \subsubsection{Failed Attempt: Superposed Model Soup}
% \ag{We can probably move this into the appendix is not}
% % Outline: Shows that naive superposition on entire models (aka superposed model soup) does not work.

% \textbf{moved it here because}: I actually didn't do experiment on superposed model soup according to the equation. I'm doing either model superposition, or superposed weight averaging (all lambda is 1 over T). The former is a baseline, the latter is also questionable because lambda is fixed. So I moved it here and maybe even remove it completely.

% As a natural extension, we follow \citet{cheung2019superposition} to superpose the weight matrices directly before summation, forming \textit{Superposed Model Soup}. Specifically, for each weight matrix $W_i$, we randomly sample an orthogonal matrix $C_i$ to rotate $W_i$ before summation:
% \begin{equation}
%     W_{\star}^{sms} = \sum_{i=1}^T\lambda_iW_iC_i
% \end{equation}
% where $\forall i\in[1,\dots,T]$, $C_iC_i^{-1}=I$. In principle, $C_i$ could be any orthogonal matrix. We found binary diagonal matrices works well with minimal memory footprint.

% \VK{would we not want to use matrices based on the task or weight vectors themselves? why random?}

% To retrieve matrix $W_k$ for task $k$, we apply the inverse of its corresponding orthogonal matrix $C_k$ onto the superposition $W_{\star}^{sms}$:
% \begin{equation}
% \hat{W}_k^{sms}=\sum_{i=1}^T\lambda_iW_iC_iC_k^{-1}=\lambda_kW_k+\sum_{i\neq k}\lambda_iW_iC_iC_k^{-1}
% \end{equation}
% Compare to equation~\ref{ms_retr}, notice the extra orthogonal transformation $C_iC_k^{-1}$ applied to each matrix in the interference term. As shown in Figure~(Some figure in appendix for sms), \ref{fig:pairwise_consine_similarity_sta}, these randomly sampled orthogonal matrices can effectively increase the mutual orthogonality among matrices and reduce the magnitude of the interference term. 

% However, despite the minimal memory usage and the promising results from online settings \citep{cheung2019superposition}, superposing entire weight matrices after training leads to miserable results as shown in Table~\ref{clip32-table}\ref{flan-t5-table}\ref{gpt2-table}. The main reason is that the random rotation cannot create perfect cancellation, but counterintuitively increase the interference magnitude as it... (roughly speaking, need plot for this and further inspection, add stuff here to motivate the transition towards superposed task arithmetic).

% \textbf{Experiments show superposed model soup can reduce the frobenius norm of the interference term, but the cosine similarity of the overall model drops from 0.99 to 0.80. Don't know how to make of it.}




% Should also leads to lower cosine similarity.

% (The empirical results are saved in "Model(Task Vector) Retrieval Difference L2 Norm")


% \begin{figure}[t]
%     \centering
%     \includegraphics[width=1.\textwidth]{images/sta_pairwise_cosine_similarity_gpt2_random_binary_diagonal_mismatch1.pdf}
%     \vspace{-4mm}
%     \caption{Pairwise cosine similarity comparison on GPT-2 models between superposed and original task vectors shifted 1-layer downwards with wraparound.}
%     \label{fig:sta_pairwise_cosine_similarity_gpt2_random_binary_diagonal_mismatch1}
%     \vspace{-1mm}
% \end{figure}


% \section{Model Merging Reformulation} \label{reformulation}
% We will now reformulate the predominant model merging algorithms into a "merge-and-retrieve" framework and expose the merging interference and their strategies to combat them. Considering a weight matrix $W_o\in\mathbb{R}^{H\times W}$ from a pre-trained model. We acquire a set of $N$ different fine-tuned versions $\{W_i\}_{i=1}^N$ for $N$ different tasks. We will use $W_\star$ to denote merged weight matrices, $\hat{W}_k$ represents the $k$th weight matrix retrieved from $W_\star$. And we define the merging interference for $W_k$ as $\Delta \hat{W}_k = \hat{W}_k-W_k$. The superscripts are acronyms of different merging algorithms.

% \subsection{Task Arithmetic}
% To merge $N$ fine-tuned weight matrices, task arithmetic uses the following formula \citep{ilharco2022editing}: 
% \begin{equation}
% W_{\star}^{ta} = W_o + \lambda\sum_{i=1}^N(W_i-W_o)
% \end{equation}
% where $\lambda\in\mathbb{R}$ is a hyper-parameter. The difference between fine-tuned weights and their pre-trained version $\{W_i-W_o\}_{i=1}^N$ are defined as task vectors.

% To perform task $k$, task arithmetic implicitly retrieves the fine-tuned weight $W_k$:
% \begin{align} \label{ta_retr}
%     \hat{W}_k^{ta}&=W_o + \lambda\sum_{i=1}^N(W_i-W_o) \nonumber\\
%     &=W_o + \lambda(W_k-W_o) + \lambda\sum_{i\neq k}(W_i-W_o) \nonumber \\
%     &=(1-\lambda)W_o + \lambda W_k + \lambda\sum_{i\neq k}(W_i-W_o)
% \end{align}

% Therefore, the merging interference for weight matrix $W_k$ is:
% \begin{equation}
%     \Delta \hat{W}_k^{ta} = \hat{W}_k^{ta} - W_k = (\lambda - 1)(W_k-W_o) + \lambda\sum_{i\neq k}(W_i-W_o)
% \end{equation}

% \subsection{Model Soup}
% Similarly, for model soup approach, we merge these $N$ weight matrices \citep{li2024scalable} with:
% \begin{equation}
% \label{e}
%     W_\star^{ms} = \sum_{i=1}^N\lambda_iW_i
% \end{equation}
% where $\{\lambda_i\in \mathbb{R}\}_{i=1}^N$ are coefficients either pre-defined \citet{izmailov2018averaging} or learned \citet{wortsman2022model}. Similar to Equation~\ref{ta_retr}, we can reformluate model soup into a retrieval framework with a well-defined merging interference when performing task $k$:
% \begin{equation}
%     \hat{W}_k^{ms} = \sum_{i=1}^N\lambda_iW_i = \lambda_kW_k + \sum_{i\neq k}\lambda_iW_i
% \end{equation}
% \begin{equation}
%     \Delta\hat{W}_k^{ms} = \hat{W}_k^{ms} - W_k = (\lambda_k-1)W_k + \sum_{i\neq k}\lambda_iW_i
% \end{equation}


% \subsection{Superposed Task Arithmetic}

% Meanwhile, superposed task arithmetic use randomly sampled binary diagonal matrices to first cast the $N$ different task vectors $\{W_i-W_o\}_{i=1}^N$ into mutually quasi-orthogonal subspace before merging them together via summation:
% \begin{equation}
%     W_{\star}^{sta} = W_o + \lambda\sum_{i=1}^N[(W_i-W_o)C_i]
% \end{equation}
% where $\forall i\in[1,\dots,N]$, $C_iC_i^{-1}=I$.

% Similarly, we can derive the retrieved weights $W_k$:
% \begin{align}
%     \hat{W}_k^{sta}&=W_o + \lambda\sum_{i=1}^N[(W_i-W_o)C_i]C_k^{-1}\nonumber\\
%     &=W_o+\lambda(W_k-W_0)C_kC_k^{-1}+\lambda\sum_{i\neq k}[(W_i-W_o)C_iC_k^{-1}] \nonumber\\
%     &=(1-\lambda)W_o+\lambda W_k+\lambda\sum_{i\neq k}[(W_i-W_o)C_iC_k^{-1}]
% \end{align}


% From equation (2) and (4) we can interpret task arithmetic methods as weighing on the pre-trained weights $W_o$ and the fine-tuned weights $W_k$ on task $k$ while balancing the interference coming from other merged weights $\{W_i\}_{i\neq k}$. Due to the specific design formula from equation (1) and (3), task arithmetic methods use the same coefficient $\lambda$ to both control the interpolation between $W_o,W_k$ and the magnitude of interference from the other weights. While to maximize model performance on task $k$, it is most ideal to set $\lambda \rightarrow 1$ to retrieve the authentic fine-tuned weight matrix $W_k$, the interference term $\sum_{i\neq k}(W_i-W_o)$ in equation (2) forces us into choosing a smaller $\lambda$ at the cost of deteriorated performance. 

% Superimposed task arithmetic overcomes this challenge by drastically dampening those interference with mutually quasi-orthogonal random binary diagonal matrices $\{C_i\}_{i=1}^N$, since $\forall i\neq j \in[1,\dots,N]$, $C_iC_j^{-1}\rightarrow 0$. Thus, we can set a $\lambda$ closer to $1$ to retrieve a more authentic $W_k$.

% (Concern: A hidden assumption here is that task vectors $\{W_i-W_o\}_{i\neq k}$ are independent to both $W_o$ and $W_k$. Intuitively it makes sense and it's also supported by cosine similarity experiment results. Should we make this assumption clear and quote the experiments here? Would quoting empirical results be enough to be rigorous?)


% \section{Task Arithmetic Reformulation}
% Considering a weight matrix $W_o\in\mathbb{R}^{A\times B}$ from a pre-trained model. We acquire a set of $N$ different fine-tuned versions $\{W_i\}_{i=1}^N$ for $N$ different tasks. To merge these $N$ weight matrices, traditional task arithmetic uses the following formula: 
% \begin{equation}
% W_{\star}^{ta} = W_o + \lambda\sum_{i=1}^N(W_i-W_o)
% \end{equation}
% where $\lambda\in\mathbb{R}$ and the difference between fine-tuned weights and their pre-trained version $\{W_i-W_o\}_{i=1}^N$ are defined as task vectors.

% To perform task $k$, traditional task arithmetic implicitly retrieves the fine-tuned weights $W_k$:
% \begin{align}
%     \hat{W}_k^{ta}&=W_o + \lambda\sum_{i=1}^N(W_i-W_o) \nonumber\\
%     &=W_o + \lambda(W_k-W_o) + \lambda\sum_{i\neq k}(W_i-W_o) \nonumber \\
%     &=(1-\lambda)W_o + \lambda W_k + \lambda\sum_{i\neq k}(W_i-W_o)
% \end{align}

% Meanwhile, superimposed task arithmetic use randomly sampled binary diagonal matrices to first cast the $N$ different task vectors $\{W_i-W_o\}_{i=1}^N$ into mutually quasi-orthogonal subspace before merging them together via summation:
% \begin{equation}
%     W_{\star}^{sta} = W_o + \lambda\sum_{i=1}^N[(W_i-W_o)C_i]
% \end{equation}
% where $\forall i\in[1,\dots,N]$, $C_iC_i^{-1}=I$.

% Similarly, we can derive the retrieved weights $W_k$:
% \begin{align}
%     \hat{W}_k^{sta}&=W_o + \lambda\sum_{i=1}^N[(W_i-W_o)C_i]\nonumber\\
%     &=W_o+\lambda(W_k-W_0)C_kC_k^{-1}+\lambda\sum_{i\neq k}[(W_i-W_o)C_iC_k^{-1}] \nonumber\\
%     &=(1-\lambda)W_o+\lambda W_k+\lambda\sum_{i\neq k}[(W_i-W_o)C_iC_k^{-1}]
% \end{align}

% From equation (2) and (4) we can interpret task arithmetic methods as weighing on the pre-trained weights $W_o$ and the fine-tuned weights $W_k$ on task $k$ while balancing the interference coming from other merged weights $\{W_i\}_{i\neq k}$. Due to the specific design formula from equation (1) and (3), task arithmetic methods use the same coefficient $\lambda$ to both control the interpolation between $W_o,W_k$ and the magnitude of interference from the other weights. While to maximize model performance on task $k$, it is most ideal to set $\lambda \rightarrow 1$ to retrieve the authentic fine-tuned weight matrix $W_k$, the interference term $\sum_{i\neq k}(W_i-W_o)$ in equation (2) forces us into choosing a smaller $\lambda$ at the cost of deteriorated performance. 

% Superimposed task arithmetic overcomes this challenge by drastically dampening those interference with mutually quasi-orthogonal random binary diagonal matrices $\{C_i\}_{i=1}^N$, since $\forall i\neq j \in[1,\dots,N]$, $C_iC_j^{-1}\rightarrow 0$. Thus, we can set a $\lambda$ closer to $1$ to retrieve a more authentic $W_k$.

% (Concern: A hidden assumption here is that task vectors $\{W_i-W_o\}_{i\neq k}$ are independent to both $W_o$ and $W_k$. Intuitively it makes sense and it's also supported by cosine similarity experiment results. Should we make this assumption clear and quote the experiments here? Would quoting empirical results be enough to be rigorous?)







\section{Experiment Setup} \label{exp_setup}

\paragraph{Datasets and Models.} 
We evaluate our methods on three sets of datasets and models provided by \textit{FusionBench}\citep{tang2024fusionbench}. For text classification and generation, we have in total eight tasks from the GLUE benchmark~\cite{wang2018glue}: CoLA, MNLI, MRPC, QNLI, QQP, RTE, and SST2. For image classification, following \citep{tang2024merging}, we use eight tasks from CLIP's test set: SUN397~\cite{sun397}, Cars~\cite{krause20133d}, RESISC45~\cite{cheng2017remote}, EuroSAT~\cite{helber2019eurosat}, SVHN~\cite{netzer2011reading}, GTSRB~\cite{stallkamp2012man}, MNIST~\cite{deng2012mnist}, and DTD~\cite{cimpoi14describing}. The model being used are: CLIP-ViT-32s \citep{radford2021learning} models with full finetuning on the vision model, Flan-T5-base full finetuning and LoRA finetunes \citep{longpre2023flan}, and GPT-2 full finetunes \citep{radford2019language}.


\paragraph{Baselines and Metrics}
We have a extensive set of baselines to compare with, thanks to the well-established model fusion benchmark \textit{FusionBench} \citep{tang2024fusionbench}. For more information about each individual baselines, please refer to \textit{FusionBench}. We also include \textit{Parameter Superposition (PSP)} \citep{cheung2019superposition} with binary diagonal matrix as an additional baseline. For evaluation metrics, our primary evaluation metric is the \textit{average accuracy} (Avg. Acc) across all tasks. This is computed by averaging the accuracies of individual tasks on their respective test sets. For the STSB task, we report Spearman's correlation coefficient. 


\paragraph{Default Setup}
In our default setup for model superposition, we use the same seed to generate binary diagonal matrix for all target layers within each model. We superpose all layers by default with random shuffling. To estimate variance, we run each experiment three times using different random seeds: 42, 43, 44.



% \subsection{Memory Cost Analysis}
%(follow \citet{wang2024localizing} Appendix C:"Let T be the number of tasks, P be the number of all parameters, P ′ be the number of trainable parameters in the model, and F be the number of frozen parameters in the model. Assuming one float parameter takes 32 bits, for each method, their respective storage cost for T tasks is calculated as:...")




% \subsection{Superposition with Different Model Architectures}
% Superpose ViT-32 with ViT-14, 

% ViTs with GPT-2 (different input space).

% Different output space: Dont have time unfortunately
% - classification (CLIP) with segmentation (Unet)
% - classification (CLIP) with DUSt3R
% - classification (CLIP) with fine-grained.





% \section{Superposition is Sparse Low-rank Approximation}
% Considering a weight matrix $W_o\in\mathbb{R}^{h\times w}$ from a pre-trained model. We acquire a set of $N$ different fine-tuned versions $\{W_i\}_{i=1}^N$ for $N$ different tasks. We will use $W_\star$ to denote merged weight matrices, $\hat{W}_k$ represents the $k$th weight matrix retrieved from $W_\star$. The superscripts are acronyms of different merging algorithms.
% We use superposed task arithmetic as an example to show superposition is a type of sparse low-rank approximation:

% \begin{equation}
%     W_{\star}^{sta} = W_o + \lambda\sum_{i=1}^N[\Delta W_iC_i] = W_o + \lambda \Delta W_\star^{sta}
% \end{equation}
% where $\forall i\in[1,\dots,N]$, $C_iC_i^{-1}=I$, $C_i\in\mathbb{R}^{w\times w}$, $\Delta W_i = W_i - W_o$ and

% \begin{equation} \label{e2}
% \Delta W_*^{sta} = [\Delta W_1 \quad \Delta W_2 \quad \cdots \quad \Delta W_N]
% \begin{bmatrix}
% C_1 \\
% C_2 \\
% \vdots \\
% C_N
% \end{bmatrix} \in \mathbb{R}^{h \times w}
% \end{equation}

% To recover $\Delta W_k$, we can do $ \Delta\hat{W}_k=\Delta W_\star C_k^{-1}$. Expanding this for all $k$, we get:

% \begin{align} \label{e3}
% &\underbrace{[\Delta \hat{W}_1 \quad \Delta \hat{W}_2 \quad \cdots \quad \Delta \hat{W}_N]}_{=\Delta \hat{W}\in\mathbb{R}^{h\times Nw}} = \Delta W_*^{sta} [C_1^{-1} \quad C_2^{-1} \quad \cdots \quad C_N^{-1}] \nonumber \\
% &= \underbrace{[\Delta W_1 \quad \Delta W_2 \quad \cdots \quad \Delta W_N]}_{=\Delta W\in\mathbb{R}^{h\times Nw}} 
% \underbrace{\begin{bmatrix}
% C_1 \\
% C_2 \\
% \vdots \\
% C_N
% \end{bmatrix}}_{=A\in\mathbb{R}^{Nw\times w}} \underbrace{[C_1^{-1} \quad C_2^{-1} \quad \cdots \quad C_N^{-1}]}_{=B\in\mathbb{R}^{w\times Nw}}\nonumber\\
% &= [\Delta W_1 \quad \Delta W_2 \quad \cdots \quad \Delta W_N]
% \begin{bmatrix}
% I & C_1C_2^{-1} & \cdots & C_1C_N^{-1} \\
% C_2C_1^{-1} & I & \cdots & C_2C_N^{-1} \\
% \vdots & \vdots & \ddots & \vdots \\
% C_NC_1^{-1} & C_NC_2^{-1} & \cdots & I
% \end{bmatrix}
% \end{align} 

% \begin{equation} \label{e1}
%     \Delta\hat{W} = \Delta W AB
% \end{equation}

% From Equation~\ref{e1} we can also treat the superposition retrievals $\Delta\hat{W}$ as a low-rank approximation of $\Delta W$. In practice, $A$ and $B$ contains diagonal matrices as blocks. So superposition is a sparse low-rank approximation.

% \subsection{Generic Model Superposition}
% Moving from the superposed task arithmetic example, now we formally discuss model superposition in its most generic form.

% Given a set of $N$ weight matrices $\{W_i\in\mathbb{R}^{h\times w}\}_{i=1}^N$, model superposition finds a set of $N$ context matrices $\{C_i\in\mathbb{R}^{w\times r}\}_{i=1}^N$ to acquire the superposed weight matrix $W_*$ with $r\in\mathbb{Z}^+$:
% \begin{equation} \label{ee1}
% W_* = [W_1 \quad W_2 \quad \cdots \quad W_N]
% \begin{bmatrix}
% C_1 \\
% C_2 \\
% \vdots \\
% C_N
% \end{bmatrix} \in \mathbb{R}^{h \times r}
% \end{equation}

% To retrieve individual weight matrices from $W_*$, model superposition constructs another set of $N$ retrieval matrices $\{R_i\in\mathbb{R}^{r\times w}\}_{i=1}^N$ such that 
% $$\forall i\in\{1,\dots,N\},\hat{W}_i=W_*R_i$$

% Expanding this for all $i$, we get:
% \begin{align} \label{e6}
% &\underbrace{[\hat{W}_1 \quad \hat{W}_2 \quad \cdots \quad \hat{W}_N]}_{=\hat{W}\in\mathbb{R}^{h\times Nw}} = W_* [R_1 \quad R_2 \quad \cdots \quad R_N] \nonumber \\
% &= \underbrace{[W_1 \quad W_2 \quad \cdots \quad W_N]}_{=W\in\mathbb{R}^{h\times Nw}} 
% \underbrace{\begin{bmatrix}
% C_1 \\
% C_2 \\
% \vdots \\
% C_N
% \end{bmatrix}}_{=C\in\mathbb{R}^{Nw\times r}} \underbrace{[R_1 \quad R_2 \quad \cdots \quad R_N]}_{=R\in\mathbb{R}^{r\times Nw}}\nonumber\\
% &= [W_1 \quad W_2 \quad \cdots \quad W_N]
% \begin{bmatrix}
% C_1R_1 & C_1R_2 & \cdots & C_1R_N \\
% C_2R_1 & C_2R_2 & \cdots & C_2R_N \\
% \vdots & \vdots & \ddots & \vdots \\
% C_NR_1 & C_NR_2 & \cdots & C_NR_N
% \end{bmatrix}
% \end{align} 
% \begin{equation}
%     \hat{W} = WCR
% \end{equation}
% where $WC\in\mathbb{R}^{h\times r}$ and $R\in\mathbb{R}^{r\times Nw}$. Thus, model superposition provides a rank-$r$ approximation of the original matrices $W$. In practice, $r<rank(W)$, and $R$ is a sparse matrix. That makes model superposition a sparse low-rank approximation.


% \subsection{Column-wise Superposition}
% Equivalently, we can treat the above mentioned process in a column-wise manner. Specifically, we can construct a permutation matrix $P\in\mathbb{R}^{Nw\times Nw}$ such that:
% \begin{equation}
%     [\text{Col}_1  \quad \text{Col}_2  \quad \dots  \quad \text{Col}_w] = [W_1  \quad W_2  \quad \dots  \quad W_N] P
% \end{equation} where \(\text{Col}_j\) consists of column $j$ from all $\{W_i\}_{i=1}^N$.

% Therefore, from equation~\ref{ee1} we get:


% \begin{align}
%     W_* &= [W_1 \quad W_2 \quad \cdots \quad W_N] PP^{-1}
% \begin{bmatrix}
% C_1 \\
% C_2 \\
% \vdots \\
% C_N
% \end{bmatrix}\nonumber \\
% &= W P P^{T} C \nonumber \\
% &= [\text{Col}_1  \quad \text{Col}_2  \quad \dots  \quad \text{Col}_w] P^TC
% \end{align}

% Similar to equation~\ref{e6}, we can get:

% \begin{align}
% &\underbrace{[\hat{\text{Col}}_1 \quad \hat{\text{Col}}_2 \quad \cdots \quad \hat{\text{Col}}_w]}_{=\hat{Col}\in\mathbb{R}^{h\times Nw}} = \underbrace{[\hat{W}_1 \quad \hat{W}_2 \quad \cdots \quad \hat{W}_N]}_{=\hat{W}\in\mathbb{R}^{h\times Nw}} P\nonumber\\ 
% &=W_*^{sta} [C_1^{-1} \quad C_2^{-1} \quad \cdots \quad C_N^{-1}]P \nonumber \\
% &= \underbrace{[\text{Col}_1 \quad \text{Col}_2 \quad \cdots \quad \text{Col}_w]}_{=\text{Col}\in\mathbb{R}^{h\times Nw}} 
% P^TCRP\nonumber\\
% &= [\text{Col}_1 \quad \text{Col}_2 \quad \cdots \quad \text{Col}_w]
% P^T\begin{bmatrix}
% C_1R_1 & C_1R_2 & \cdots & C_1R_N \\
% C_2R_1 & C_2R_2 & \cdots & C_2R_N \\
% \vdots & \vdots & \ddots & \vdots \\
% C_NR_1 & C_NR_2 & \cdots & C_NR_N
% \end{bmatrix}P
% \end{align}
% \begin{equation}
%     \hat{Col} = Col P^TCRP
% \end{equation}

% The same argument follows.

% \subsection{Sparsity Lower Bound Against SVD Alternative}
% As shown in equation~\ref{e1}, superposition is a type of sparse low rank decomposition: $$\Delta \hat{W}^{sup}=\Delta W AB = A^{sup}B^{sup}$$ where $A^{sup}=\Delta WA\in\mathbb{R}^{h\times r^{sup}}$ and $B^{sup} = B\in\mathbb{R}^{r^{sup}\times Nw}$ are a dense and sparse matrix, respectively. 

% Meanwhile, singular value decomposition (SVD), according to the Eckart-Young theorem, provides the optimal rank-r approximation of a matrix in terms of Frobenius norm. We can similarly approximate $\Delta W$ with SVD:
% $$\Delta\hat{W}^{svd}=A^{svd}B^{svd}$$ where $A^{svd}\in\mathbb{R}^{h\times r^{svd}}$ and $B^{svd} \in\mathbb{R}^{r^{svd}\times Nw}$ are both dense matrices.

% To compare the memory footprint in byte of the two methods, let's assume all matrices use $x$ bytes to store each element. To store the sparse matrix $B^{sup}$, we use the Compressed Sparse Row (CSR) format. In CSR format, a matrix is stored using three arrays:
% \begin{enumerate}
%     \item Values array: Stores the non-zero elements.
%     \item Column indices array: Stores the column index of each non-zero element.
%     \item Row pointer array: Stores the cumulative count of non-zero elements at the start of each row.
% \end{enumerate}
% And we use $x$ bytes to store indices.

% Therefore, the total storage for superposition is:
% \begin{align}
%     S^{sup} &= x[hr^{sup}+(1-p)r^{sup}Nw] + x[hr^{sup}+(1-p)r^{sup}Nw] + x(h+1) \nonumber \\
%     &= xr^{sup}[h+2(1-p)Nw] + x(h+1)
% \end{align} where $p$ is the sparsity of matrix $B^{sup}$.

% For SVD, we can get:
% \begin{equation}
%     S^{svd} = xr^{svd}(h+Nw)
% \end{equation}

% When $S^{sup}<S^{svd}$, we have
% \begin{align}
%     &S^{sup}<S^{svd} \nonumber \\
%     &xr^{sup}[h+2(1-p)Nw] + x(h+1) < xr^{svd}(h+Nw) \nonumber \\
%     &p>\frac{r^{sup}(h+2Nw)-r^{svd}(h+Nw)+h+1}{2Nwr^{sup}}
% \end{align}

% To get a sense of how sparse $B^{sup}$ needs to be for $S^{sup}<S^{svd}$, consider $h=3072$, $Nw=6144$, and $r^{sup}=r^{svd}=768$. Then $p>0.5$.



%\ag{Find theorem from fields like VSAs that say something like "applying random orthogonal matrices to two high dimensional vectors increase their orthogonality". reduce our setup to theirs, show that we are a special case. very likely to reduce cosine similarity. done below}

% \section{Random Matrices in High Dimneional Space}

% In the following proof, we will provide some motivation about why applying random matrices to similar vectors can lead to them to being more orthogonal in high dimensional space.

% Let $\mathbf{v}_1, \mathbf{v}_2 \in \mathbb{R}^d$ be two arbitrary vectors, and let $\mathbf{O} \in \mathbb{R}^{d \times d}$ be a random orthogonal matrix. Consider the transformed vectors $\mathbf{v}_1' = \mathbf{O} \mathbf{v}_1$ and $\mathbf{v}_2' = \mathbf{O} \mathbf{v}_2$. We aim to show that the cosine similarity between $\mathbf{v}_1'$ and $\mathbf{v}_2'$ decreases as $d$ increases.

% %\paragraph{Step 1: Expected Cosine Similarity.}
% The cosine similarity between the transformed vectors is given by:
% \[
% \cos(\mathbf{v}_1', \mathbf{v}_2') = \frac{\langle \mathbf{v}_1', \mathbf{v}_2' \rangle}{\|\mathbf{v}_1'\| \|\mathbf{v}_2'\|}.
% \]
% Since $\mathbf{O}$ is orthogonal, the norms of the vectors are preserved, i.e., $\|\mathbf{v}_1'\| = \|\mathbf{v}_1\|$ and $\|\mathbf{v}_2'\| = \|\mathbf{v}_2\|$. Thus, we focus on the inner product $\langle \mathbf{v}_1', \mathbf{v}_2' \rangle$.

% %\paragraph{Step 2: Random Matrix Effect.}
% The matrix $\mathbf{O}$ is drawn from the Haar distribution over the orthogonal group, which means that the entries of $\mathbf{v}_1'$ and $\mathbf{v}_2'$ become uncorrelated as $d$ increases. By properties of random orthogonal matrices, the expected value of the inner product is:
% \[
% \mathbb{E}[\langle \mathbf{v}_1', \mathbf{v}_2' \rangle] = 0.
% \]
% This is because the components of $\mathbf{v}_1'$ and $\mathbf{v}_2'$ behave like independent random variables with zero mean in high dimensions. %\paragraph{Step 3: Variance and High-Dimensional Behavior.} 
% In high dimensions, the variance of the inner product $\langle \mathbf{v}_1', \mathbf{v}_2' \rangle$ is proportional to $1/d$, meaning that as $d \to \infty$, the inner product tends to zero with high probability:
% \[
% \langle \mathbf{v}_1', \mathbf{v}_2' \rangle \approx 0 \quad \text{as} \quad d \to \infty.
% \]
% Thus, the cosine similarity also tends to zero:
% \[
% \mathbb{P}(\cos(\mathbf{v}_1', \mathbf{v}_2') \approx 0) \to 1 \quad \text{as} \quad d \to \infty.
% \]

% Therefore, applying a random orthogonal matrix $\mathbf{O}$ to two high-dimensional vectors $\mathbf{v}_1$ and $\mathbf{v}_2$ leads to an increase in orthogonality, as the cosine similarity between the transformed vectors decreases to zero with high probability as the dimensionality increases.



% \subsection{Theoretical Insights: Blessing of Dimensionality}

% Our proposed method for task vector superposition and random layer shuffling relies on high-dimensional geometric properties, commonly referred to as the \textit{blessing of dimensionality}. Below, we provide theoretical justification for the reduction in interference and improvement in task retrieval.

% % \paragraph{Random Orthogonal Transformations.}
% In high-dimensional spaces, random orthogonal transformations increase the likelihood of vectors being nearly orthogonal. Formally, let $\mathbf{T}_i \in \mathbb{R}^d$ represent task vectors, and let $\mathbf{C}_i$ be a random orthogonal matrix. Applying $\mathbf{C}_i$ to $\mathbf{T}_i$ leads to vectors that have lower cosine similarity:
% \[
% \cos(\mathbf{T}_i, \mathbf{T}_j) \quad \text{becomes} \quad \cos(\mathbf{T}_i \mathbf{C}_i, \mathbf{T}_j \mathbf{C}_j),
% \]
% where the new cosine similarity between transformed vectors $\mathbf{T}_i \mathbf{C}_i$ and $\mathbf{T}_j \mathbf{C}_j$ is much smaller due to the high-dimensional nature of $\mathbb{R}^d$.

% % \paragraph{Cosine Similarity and Dimensionality.}
% As dimensionality increases, random vectors in $\mathbb{R}^d$ tend to be almost orthogonal. This follows from the \textit{Johnson-Lindenstrauss Lemma} from ~\cite{johnson1986extensions}, which states that random projections into high-dimensional spaces approximately preserve pairwise distances:
% \[
% \forall i \neq j, \quad \mathbb{P}\left( \cos(\mathbf{T}_i, \mathbf{T}_j) \approx 0 \right) \to 1 \quad \text{as} \quad d \to \infty.
% \]
% Thus, random orthogonal matrices $\mathbf{C}_i$ ensure low interference between task vectors in task arithmetic.

% % \paragraph{Interference Reduction.}
% By shuffling layers or applying random orthogonal matrices, we reduce interference in task vector superposition. The interference term:
% \[
% \sum_{i \neq k} \cos(\mathbf{T}_i, \mathbf{T}_k)
% \]
% becomes:
% \[
% \sum_{i \neq k} \cos(\mathbf{T}_i \mathbf{C}_i, \mathbf{T}_k \mathbf{C}_k),
% \]
% which is significantly smaller due to the orthogonality induced by high-dimensional transformations. This leads to improved task retrieval and reduced mutual interference between task vectors.

% % \paragraph{Orthogonality Preservation.}
% Orthogonal matrices preserve the norm of the original vectors:
% \[
% \|\mathbf{T}_i\| = \|\mathbf{T}_i \mathbf{C}_i\|,
% \]
% ensuring that task vectors retain their original magnitudes while becoming less aligned, further contributing to the reduction of interference.

% The \textit{blessing of dimensionality} guarantees that random transformations in high-dimensional space lead to increased orthogonality between task vectors, reducing interference and improving the retrieval of merged models.
